# Supplementary material for: Dual Prompting Image Restoration with Diffusion Transformers
Source: arXiv:2504.17825 source file (2025-04-24)
Supplement: Supplementary file 1 [file 7_suppl.tex]

\clearpage

\setcounter{section}{0}
\setcounter{equation}{0}
\setcounter{page}{1}
\maketitlesupplementary
Sec. \ref{sec:detailmethod} provides a more detailed explanation of our dual prompting approach, specifically dissecting the generation of $c_{dual}$. In Set. \ref{sec:detailtrain}, we supplement more details on VAE and model training.  Sec. \ref{sec:visual} shows more visual examples for qualitative comparisons. The results of a user
study in the form of voting results and assessments of image quality at the pixel level in Sec. \ref{sec:user}.
% 
% Having the supplementary compiled together with the main paper means that:
% % 
% \begin{itemize}
% \item The supplementary can back-reference sections of the main paper, for example, we can refer to \cref{sec:intro};
% \item The main paper can forward reference sub-sections within the supplementary explicitly (e.g. referring to a particular experiment); 
% \item When submitted to arXiv, the supplementary will already included at the end of the paper.
% \end{itemize}
% % 
% To split the supplementary pages from the main paper, you can use \href{https://support.apple.com/en-ca/guide/preview/prvw11793/mac#:~:text=Delete%20a%20page%20from%20a,or%20choose%20Edit%20%3E%20Delete).}{Preview (on macOS)}, \href{https://www.adobe.com/acrobat/how-to/delete-pages-from-pdf.html#:~:text=Choose%20%E2%80%9CTools%E2%80%9D%20%3E%20%E2%80%9COrganize,or%20pages%20from%20the%20file.}{Adobe Acrobat} (on all OSs), as well as \href{https://superuser.com/questions/517986/is-it-possible-to-delete-some-pages-of-a-pdf-document}{command line tools}.
